# Supplementary material for: Certifying steady-state properties of open quantum systems
Source: arXiv:2410.13646 source file (2025-06-17)
Supplement: Supplementary file 1 [file suppmat.pdf]

# Supplemental material for "Certifying steady-state properties of open quantum systems"

## SYMMETRY CONSTRAINTS

If we know that the system takes some form, there can be additional constraints we can exploit. Here, let us assume the system has a unique steady state (non-zero Liouvillian gap). For example, if we know that the system is invariant under some swap of qubits, we can further constrain that their respective expectation values should be equal. For instance, if we have a simple two-by-two grid system, such that the two leftmost qubits are connected to the hot bath and the two rightmost qubits are connected to the cold bath, we can enforce that the expectation values of the leftmost qubits are equal, as well as their combined expectation values with the rightmost qubits, following the symmetries. Such constraints are "for free" in that they add negligible computational cost, but can often improve the bounds by a non-negligible amount.

## PERSPECTIVES: HEAT CURRENT CONSTRAINTS/CERTIFICATION

Let us consider a non-equilibrium steady state obtained by connecting the system to a hot bath and to a cold bath and examine the heat currents, either from one of the baths or between two neighbouring spins such as in Fig. 1(a) of the main text. More specifically, assuming we have a Lindbladian in the form

$$\mathcal{L}\left(\rho\right) = -i\left[H, \rho\right] + \mathcal{L}_h(\rho) + \mathcal{L}_c(\rho)\,, \tag{1}$$

where $\mathcal{L}_{h(c)}$ is the dissipator associated to the hot(cold) bath, the heat current supplied by the hot bath at steady state is given by [1]

$$J_h = \langle \mathcal{L}_h^\dagger(H) \rangle_{ss}\ . \tag{2}$$

Such an expression can then be used either as an objective or we can impose a constraint on it. Using it as an objective we can, e.g., attempt to certify that the flow of energy implied by the considered Lindbladian is from hot to cold (positive sign for $J_h = -J_c$), i.e., obeying the second law of thermodynamics. Put differently, in principle it is possible to identify Lindbladians violating the second law, as happening in the well known example of the local master equation under some conditions [2]. Meanwhile, under the guarantee that the second law is satisfied for the Lindbladian under analysis, using the second law as a constraint (e.g., such that all pairwise flows from the hot to the cold should be positive) could theoretically result in better constraining, although in practice we are yet to find a system in which this significantly helps.

## DATA TABLES

We report here further numerical results on the open quantum systems analysed in the main text. Specifically, we present in Table I the various bounds given by different combinations of constraints for the two-qubit model depicted in Fig. 1(a) and in Table II specific results of different combinations of constraints for the 2D ladder of Fig. 1(c).

| Moment Matrix | Linear | State Reconstruction | Symmetry | Bounded Interval | Time |
|---|---|---|---|---|---|
| None | level 1 (6) | None | None | [-0.000001, 0.001167] (8.83%) | 0.03s |
| level 1 (7x7) | level 1 (6) | None | None | [-0.000001, 0.001167] (8.83%) | 0.04s |
| None | level 2 (15) | None | None | [0.000209, 0.000209] (0.0%) | 0.05s |
| None | auto (6) | None | None | [0.000209, 0.000209] (0.0%) | 0.03s |

Table I. Bounds on the average heat current for the two-qubit system (Figure 1(a)), for a variety of possible constraints (the first four columns). The bounds given are the strict lower and upper bounds for the heat current in the steady state, whilst the percentages represent the fraction of the trivial region that the bounds cover. The other values in parentheses are either the size of matrix or number of constraints added. The time taken for this case is almost entirely setup time, hence the lack of change with more/less constraints. The interesting point of note here is that we do not need all 15 constraints to exactly solve the system - only 6 suffice. This system is described by equations (8), (9) and (10) in the main text, with parameters $\gamma_c = 0.011$, $\gamma_h = 0.001$, $g = 0.0016$, $T_h = 1.0$, $T_c = 0.1$, $\delta = 0.005$, $\epsilon_h = 1.0$.

| Moment Matrix | Linear | State Reconstruction | Symmetry | Bounded Interval | Time |
|---|---|---|---|---|---|
| None | auto (1000) | None | None | [-0.978822, 0.307664] (64.32%) | 0.96s |
| auto (101x101) | auto (10000) | None | None | [-0.882218, 0.174893] (52.86%) | 37.48s |
| None | auto (10000) | all 4-site (386x16x16) | None | [-0.853122, -0.128460] (36.23%) | 40.92s |
| None | auto (10000) | all 4-site (386x16x16) | yes (5) | [-0.853120, -0.128461] (36.23%) | 41.09s |
| None | auto (50000) | all 4-site (386x16x16) | yes (5) | [-0.852470, -0.132688] (35.99%) | 25m37s |
| None | auto (100000) | all 4-site (386x16x16) | yes (5) | [-0.852460, -0.132781] (35.98%) | 147m35s |

Table II. Bounds on the average magnetisation for the 2x5 ladder chain (Figure 1(c)), for a variety of possible constraints (the first four columns). The bounds given are the strict lower and upper bounds for the heat current in the steady state, whilst the percentages represent the fraction of the full $[-1, 1]$ region that the bounds cover. The other values in parentheses are either the size of matrix or number of constraints added. The system is described by Eq. (13) in the main text, with parameters $\gamma_c = 0.011$, $\gamma_h = 0.001$, $g = 0.0016$, $T_h = 1.0$, $T_c = 0.1$, $\epsilon_h = 1.0$, $\epsilon_c = 1.005$, $\epsilon_i = (\epsilon_h + \epsilon_c)/2$ for $i \neq h$ and $i \neq c$.

[1] R. Alicki and R. Kosloff, Thermodynamics in the Quantum Regime: Fundamental Aspects and New Directions , 1 (2018).
[2] A. Levy and R. Kosloff, Europhysics Letters **107**, 20004 (2014).
